# Supplementary material for: The Quest For Highly Accurate Excitation Energies: A Computational Perspective
Source: arXiv:2001.00416 source file (2020-01-31)
Supplement: Supplementary file 1 [file SI.pdf]

**Table S1: Non-exhaustive list of previous benchmark studies of wavefunction (and BSE) methods. We report the method, the year of publication, the characteristics of the set (both number of excited states and nature of the molecules), the benchmark set, the MAE (in eV), and the reference values. S ans T stands for singlet and triplet respectively, and are specified only when the separated statistics are provided in the original work. Further details can be found in the corresponding studies (references provided).**

| Method | Year | No. of ES | No. of molecules | Benchmark set | MAE (eV) | Ref. |
|---|---|---|---|---|---|---|
| BSE@ev$GW$ | 2015 | 91 | 28 (medium-size organic) | Th. $E_{\text{abs}}^{\text{vert}}$ (Thiel's TBE-2) | 0.25 | 1 |
| | 2015 | 80 | 80 (organic dyes) | Exp. $E^{\text{0-0}}$ (solvated) | 0.19/0.15[a] | 2 |
| | 2017 | 23 | 18 (various) | Exp. excitation energies | 0.18 | 3 |
| | 2017 | 62 (T) | 20 (medium-size organic) | Th. $E_{\text{abs}}^{\text{vert}}$ (CC3) | 0.58 | 4 |
| | 2018 | 104 (S) | 28 (medium-size organic ) | Th. $E_{\text{abs}}^{\text{vert}}$ (CC3) | 0.26 | 5 |
| | 2018 | 63 (T) | 20 (medium-size organic) | Th. $E_{\text{abs}}^{\text{vert}}$ (CC3) | 0.84 | 5 |
| CIS | 1995 | 6 | 6 (diatomics) | Exp. $E^{\text{adia}}$ | 0.73 | 6 |
| | 2002 | 34 | 28 (mostly di/triatomics) | Exp. $E^{\text{adia}}$ and $E^{\text{0-0}}$ | 0.63 | 7 |
| | 2005 | 19 | 4 (diatomics) | Exp. $E^{\text{adia}}$ | 0.57 | 8 |
| | 2007 | 32 | 22 (diverse) | Exp. $E^{\text{0-0}}$ | 0.71 | 9 |
| | 2009 | 20 | 29 (mostly di/triatomics) | Exp. $E^{\text{adia}}$ and $E^{\text{0-0}}$ | 0.58 | 10 |
| | 2010 | 69 | 11 (medium-size organic) | Exp. excitation energies | 1.07 | 11 |
| | 2010 | 12 | 12 (organic dyes) | Exp. $E^{\text{0-0}}$ (solvated) | 0.77 | 12 |
| | 2011 | 91 | 109 (diverse) | Exp. $E^{\text{0-0}}$ | 0.98 | 13 |
| | 2013 | 7 | 7 (organic dyes) | Exp. $E^{\text{0-0}}$ (solvated) | 0.75 | 14 |
| | 2014 | 79 | 96 (various) | Exp. $E^{\text{0-0}}$ | 0.88 | 15 |
| | 2014 | 29 | 15 (small radicals) | Exp. $E^{\text{0-0}}$ | 1.75 | 16 |
| | 2017 | 66 | 46 (aromatics) | Exp. $E^{\text{0-0}}$ | 1.08 | 17 |
| CIS(D) | 1995 | 6 | 6 (diatomics) | Exp. $E^{\text{adia}}$ | 0.27 | 6 |
| | 2004 | 32 | 22 (diverse) | Exp. $E^{\text{0-0}}$ | 0.19 | 18 |
| | 2005 | 19 | 4 (diatomics) | Exp. $E^{\text{adia}}$ | 0.26 | 8 |
| | 2007 | 32 | 22 (diverse) | Exp. $E^{\text{0-0}}$ | 0.22 | 9 |
| | 2010 | 69 | 11 (medium-size organic) | Exp. excitation energies | 0.49 | 11 |
| | 2010 | 12 | 12 (organic dyes) | Exp. $E^{\text{0-0}}$ (solvated) | 0.25 | 12 |
| | 2015 | 80 | 80 (organic dyes) | Exp. $E^{\text{0-0}}$ (solvated) | 0.18/0.26[a] | 2 |
| | 2018 | 106 | 18 (small compounds) | Th. $E_{\text{abs}}^{\text{vert}}$ (FCI) | 0.25 | 19 |
| | 2020 | 221 | 27 (medium-size organic) | Th. $E_{\text{abs}}^{\text{vert}}$ (FCI, CCSDTQ, CCSDT) | 0.23 | 20 |
| ADC(2) | 2002 | 43 | 4 (small) | Th. $E_{\text{abs}}^{\text{vert}}$ (FCI) | 0.64 | 21 |
| | 2005 | 19 | 4 (diatomics) | Exp. $E^{\text{adia}}$ | 0.21 | 8 |
| | 2013 | 66 | 46 (aromatics) | Exp. $E^{\text{0-0}}$ | 0.08 | 22 |
| | 2014 | 104 | 28 (medium-size organic) | Th. $E_{\text{abs}}^{\text{vert}}$ (Thiel's TBE) | 0.29 | 23 |
| | 2015 | 80 | 80 (organic dyes) | Exp. $E^{\text{0-0}}$ (solvated) | 0.22/0.14[a] | 2 |
| | 2018 | 106 | 18 (small compounds) | Th. $E_{\text{abs}}^{\text{vert}}$ (FCI) | 0.21 | 19 |
| | 2020 | 101 | 94 (medium-size organic) | Exp. $E^{\text{0-0}}$ | 0.16 | 24 |
| | 2020 | 328 | 45 (1–6 non-H atoms) | Th. $E_{\text{abs}}^{\text{vert}}$ (FCI, CCSDTQ, CCSDT) | 0.16 | 24 |
| | 2020 | 218 | 27 (medium-size organic) | Th. $E_{\text{abs}}^{\text{vert}}$ (FCI, CCSDTQ, CCSDT) | 0.14 | 20 |
| ADC(3) | 2002 | 43 | 4 (small) | Th. $E_{\text{abs}}^{\text{vert}}$ (FCI) | 0.17 | 21 |
| | 2014 | 104 | 28 (medium-size organic) | Th. $E_{\text{abs}}^{\text{vert}}$ (Thiel's TBE) | 0.24 | 23 |
| | 2018 | 106 | 18 (small compounds) | Th. $E_{\text{abs}}^{\text{vert}}$ (FCI) | 0.23 | 19 |
| | 2020 | 101 | 94 (medium-size organic) | Exp. $E^{\text{0-0}}$ | 0.18 | 24 |
| | 2020 | 328 | 45 (1–6 non-H atoms) | Th. $E_{\text{abs}}^{\text{vert}}$ (FCI, CCSDTQ, CCSDT) | 0.21 | 24 |
| CC2 | 2002 | 43 | 4 (small) | Th. $E_{\text{abs}}^{\text{vert}}$ (FCI) | 0.53 | 21 |
| | 2003 | 20 | 29 (mostly di/triatomics) | Exp. $E^{\text{adia}}$ and $E^{\text{0-0}}$ | 0.17 | 25 |
| | 2005 | 19 | 4 (diatomics) | Exp. $E^{\text{adia}}$ | 0.16 | 8 |
| | 2008 | 26 | 19 (di/triatomics) | Exp. $E^{\text{adia}}$ and $E^{\text{0-0}}$ | 0.17 | 26 |
| | 2008 | 32 | 22 (diverse) | Exp. $E^{\text{0-0}}$ | 0.14 | 26 |
| | 2008 | 152 (S) | 28 (medium-size organic) | Th. $E_{\text{abs}}^{\text{vert}}$ (CASPT2) | 0.32 | 27 |
| | 2008 | 71 (T) | 20 (medium-size organic) | Th. $E_{\text{abs}}^{\text{vert}}$ (CASPT2) | 0.19 | 27 |
| | 2009 | 20 | 29 (mostly di/triatomics) | Exp. $E^{\text{adia}}$ and $E^{\text{0-0}}$ | 0.18 | 10 |
| | 2011 | 15 | 15 (diverse) | Exp. $E^{\text{0-0}}$ | 0.17 | 13 |
| | 2013 | 66 | 46 (aromatics) | Exp. $E^{\text{0-0}}$ | 0.07 | 22 |
| | 2014 | 79 | 96 (various) | Exp. $E^{\text{0-0}}$ | 0.19 | 15 |

Continued on next page

| Method | Year | No. of ES | No. of molecules | Benchmark set | MAE (eV) | Ref. |
|---|---|---|---|---|---|---|
| | 2015 | 80 | 80 (organic dyes) | Exp. $E^{0\text{-}0}$ (solvated) | 0.16/0.13[a] | 2 |
| | 2016 | 132 | 25 (medium-size organic) | Th. $E^{\text{vert}}_{\text{abs}}$ (CC3) | 0.22 | 28 |
| | 2017 | 66 | 46 (aromatics) | Exp. $E^{0\text{-}0}$ | 0.11 | 17 |
| | 2018 | 106 | 18 (small compounds) | Th. $E^{\text{vert}}_{\text{abs}}$ (FCI) | 0.22 | 19 |
| | 2018 | 35 | 31 (medium-size organic) | Exp. $E^{0\text{-}0}$ | 0.08 | 29 |
| | 2020 | 101 | 94 (medium-size organic) | Exp. $E^{0\text{-}0}$ | 0.10 | 24 |
| | 2020 | 328 | 45 (1–6 non-H atoms) | Th. $E^{\text{vert}}_{\text{abs}}$ (FCI, CCSDTQ, CCSDT) | 0.17 | 24 |
| | 2020 | 223 | 27 (medium-size organic) | Th. $E^{\text{vert}}_{\text{abs}}$ (FCI, CCSDTQ, CCSDT) | 0.15 | 20 |
| CCSD | 1995 | 6 | 6 (diatomics) | Exp. $E^{\text{adia}}$ | 0.19 | 6 |
| | 2002 | 43 | 4 (small) | Th. $E^{\text{vert}}_{\text{abs}}$ (FCI) | 0.15 | 21 |
| | 2005 | 19 | 4 (diatomics) | Exp. $E^{\text{adia}}$ | 0.20 | 8 |
| | 2008 | 152 (S) | 28 (medium-size organic) | Th. $E^{\text{vert}}_{\text{abs}}$ (CASPT2) | 0.50 | 27 |
| | 2008 | 71 (T) | 20 (medium-size organic) | Th. $E^{\text{vert}}_{\text{abs}}$ (CASPT2) | 0.16 | 27 |
| | 2010 | 69 | 11 (medium-size organic) | Exp. excitation energies | 0.27 | 11 |
| | 2016 | 132 | 25 (medium-size organic) | Th. $E^{\text{vert}}_{\text{abs}}$ (CC3) | 0.15 | 28 |
| | 2017 | 23 | 18 (various) | Exp. excitation energies | 0.31 | 3 |
| | 2018 | 106 | 18 (small compounds) | Th. $E^{\text{vert}}_{\text{abs}}$ (FCI) | 0.08 | 19 |
| | 2018 | 35 | 31 (medium-size organic) | Exp. $E^{0\text{-}0}$ | 0.21 | 29 |
| | 2020 | 223 | 27 (medium-size organic) | Th. $E^{\text{vert}}_{\text{abs}}$ (FCI, CCSDTQ, CCSDT) | 0.13 | 20 |
| CC3 | 2002 | 43 | 4 (small) | Th. $E^{\text{vert}}_{\text{abs}}$ (FCI) | 0.02 | 21 |
| | 2005 | 19 | 4 (diatomics) | Exp. $E^{\text{adia}}$ | 0.04 | 8 |
| | 2008 | 121 (S) | 28 (medium-size organic) | Th. $E^{\text{vert}}_{\text{abs}}$ (CASPT2) | 0.20 | 27 |
| | 2008 | 71 (T) | 20 (medium-size organic) | Th. $E^{\text{vert}}_{\text{abs}}$ (CASPT2) | 0.08 | 27 |
| | 2018 | 35 | 31 (medium-size organic) | Exp. $E^{0\text{-}0}$ | 0.02 | 29 |
| | 2018 | 106 | 18 (small compounds) | Th. $E^{\text{vert}}_{\text{abs}}$ (FCI) | 0.04 | 19 |
| | 2019 | 119 | 109 (diverse) | Exp. $E^{0\text{-}0}$ | 0.03 | 30 |
| | 2020 | 101 | 94 (medium-size organic) | Exp. $E^{0\text{-}0}$ | 0.04 | 24 |
| | 2020 | 328 | 45 (1–6 non-H atoms) | Th. $E^{\text{vert}}_{\text{abs}}$ (FCI, CCSDTQ, CCSDT) | 0.02 | 24 |
| | 2020 | 223 | 27 (medium-size organic) | Th. $E^{\text{vert}}_{\text{abs}}$ (FCI, CCSDTQ, CCSDT) | 0.01 | 20 |
| CCSDT | 2018 | 104 | 18 (small compounds) | Th. $E^{\text{vert}}_{\text{abs}}$ (FCI) | 0.03 | 19 |
| CCSDTQ | 2018 | 73 | 18 (small compounds) | Th. $E^{\text{vert}}_{\text{abs}}$ (FCI) | 0.01 | 19 |
| CASPT2 | 2013 | 121 | 28 (medium-size organic) | Th. $E^{\text{vert}}_{\text{abs}}$ (CC3) | 0.21 | 31 |
| | 2014 | 29 | 15 (small radicals) | Exp. $E^{0\text{-}0}$ | 0.12 | 16 |
| | 2016 | 23 | 18 (various) | Exp. excitation energies | 0.21 | 32 |
| | 2017 | 124 | 13 (di and triatomics) | Th. $E^{\text{vert}}_{\text{abs}}$ (FCI) | 0.10/0.11[b] | 33 |
| | 2017 | 130 | 28 (medium-size organic) | Exp. excitation energies | 0.25–0.33[b] | 33 |
| (PC-)NEVPT2 | 2013 | 121 | 28 (medium-size organic) | Th. $E^{\text{vert}}_{\text{abs}}$ (CC3) | 0.28 | 31 |
| | 2020 | 223 | 27 (medium-size organic) | Th. $E^{\text{vert}}_{\text{abs}}$ (FCI, CCSDTQ, CCSDT) | 0.13 | 20 |

[a] Depending on the selected solvent model: LR/cLR.

[b] With the largest considered basis set, 6-311G, using (or not) various IPEA, see the original work.

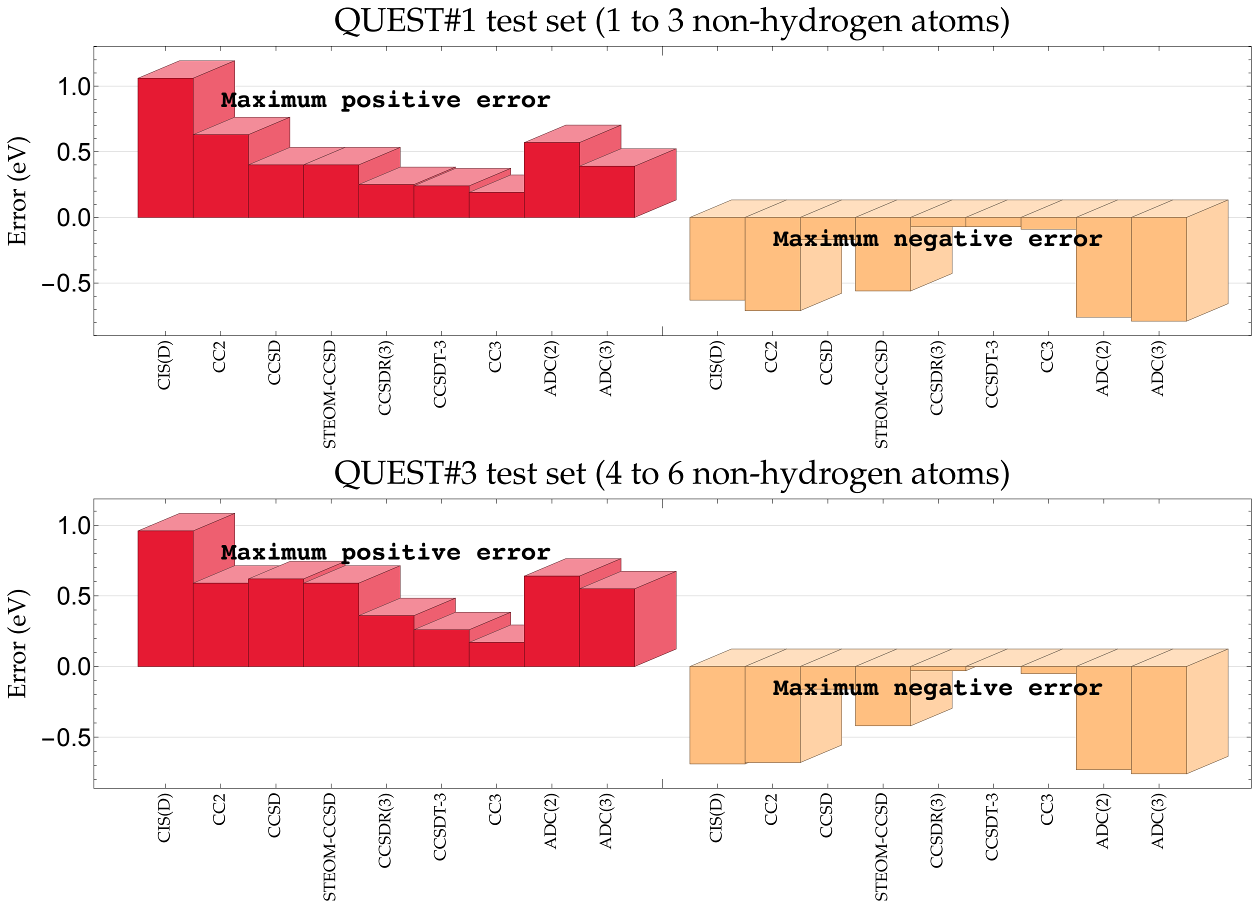


Figure S1: Maximum positive and maximum negative errors (in eV) for the QUEST#1 and QUEST#3 sets of excitation energies with respect to the TBE/*aug*-cc-pVTZ reference values (as described in Refs. 19,20) for various methods.

## REFERENCES


(1) Jacquemin, D.; Duchemin, I.; Blase, X. Benchmarking the Bethe-Salpeter Formalism on a Standard Organic Molecular Set. *J. Chem. Theory Comput.* **2015**, *11*, 3290–3304.

(2) Jacquemin, D.; Duchemin, I.; Blase, X. 0–0 Energies Using Hybrid Schemes: Benchmarks of TD-DFT, CIS(D), ADC(2), CC2, and BSE/GW formalisms for 80 Real-Life Compounds. *J. Chem. Theory Comput.* **2015**, *11*, 5340–5359.

(3) Jacquemin, D.; Duchemin, I.; Blase, X. Is the Bethe–Salpeter Formalism Accurate for Excitation Energies? Comparisons with TD-DFT, CASPT2, and EOM-CCSD. *J. Phys. Chem. Lett.* **2017**, *8*, 1524–1529.

(4) Jacquemin, D.; Duchemin, I.; Blondel, A.; Blase, X. Benchmark of Bethe-Salpeter for Triplet Excited-States. *J. Chem. Theory Comput.* **2017**, *13*, 767–783.

(5) Gui, X.; Holzer, C.; Klopper, W. Accuracy Assessment of *GW* Starting Points for Calculating Molecular Excitation Energies Using the Bethe–Salpeter Formalism. *J. Chem. Theory Comput.* **2018**, *14*, 2127–2136.

(6) Stanton, J. F.; Gauss, J. Analytic Energy Derivatives for the Equation-of-Motion Coupled-Cluster Method: Algebraic Expressions, Implementation and Application to the $S_1$ State of HFCO. *Theor. Chim. Acta* **1995**, *91*, 267–289.

(7) Furche, F.; Ahlrichs, R. Adiabatic Time-Dependent Density Functional Methods for Excited States Properties. *J. Chem. Phys.* **2002**, *117*, 7433–7447.

(8) Hättig, C. In *Response Theory and Molecular Properties (A Tribute to Jan Linderberg and Poul Jørgensen)*; Jensen, H. A., Ed.; Advances in Quantum Chemistry; Academic Press, 2005; Vol. 50; pp 37–60.

(9) Rhee, Y. M.; Head-Gordon, M. Scaled Second-Order Perturbation Corrections to Configuration Interaction Singles: Efficient and Reliable Excitation Energy Methods. *J. Phys. Chem. A* **2007**, *111*, 5314–5326.

(10) Rhee, Y. M.; Casanova, D.; Head-Gordon, M. Performance of Quasi-Degenerate Scaled Opposite Spin Perturbation Corrections to Single Excitation Configuration Interaction for Excited State Structures and Excitation Energies with Application to the Stokes Shift of 9-Methyl-9,10-dihydro-9-silaphenanthrene. *J. Phys. Chem. A* **2009**, *113*, 10564–10576.

(11) Caricato, M.; Trucks, G. W.; Frisch, M. J.; Wiberg, K. B. Electronic Transition Energies: A Study of the Performance of a Large Range of Single Reference Density Functional and Wave Function Methods on Valence and Rydberg States Compared to Experiment. *J. Chem. Theory Comput.* **2010**, *6*, 370–383.

(12) Goerigk, L.; Grimme, S. Assessment of TD-DFT Methods and of Various Spin Scaled CIS$_n$D and CC2 Versions for the Treatment of Low-Lying Valence Excitations of Large Organic Dyes. *J. Chem. Phys.* **2010**, *132*, 184103.

(13) Send, R.; Kühn, M.; Furche, F. Assessing Excited State Methods by Adiabatic Excitation Energies. *J. Chem. Theory Comput.* **2011**, *7*, 2376–2386.

(14) Chantzis, A.; Laurent, A. D.; Adamo, C.; Jacquemin, D. Is the Tamm-Dancoff Approximation Reliable for the Calculation of Absorption and Fluorescence Band Shapes? *J. Chem. Theory Comput.* **2013**, *9*, 4517–4525.

(15) Fang, C.; Oruganti, B.; Durbeej, B. How Method-Dependent Are Calculated Differences Between Vertical, Adiabatic and 0-0 Excitation Energies? *J. Phys. Chem. A* **2014**, *118*, 4157–4171.

(16) Barnes, L.; Abdul-Al, S.; Allouche, A.-R. TDDFT Assessment of Functionals for Optical 0–0 Transitions in Small Radicals. *J. Phys. Chem. A* **2014**, *118*, 11033–11046, PMID: 25350349.

(17) Oruganti, B.; Fang, C.; Durbeej, B. Assessment of a Composite CC2/DFT Procedure for Calculating 0–0 Excitation Energies of Organic Molecules. *Mol. Phys.* **2016**, *114*, 3448–3463.

(18) Grimme, S.; Izgorodina, E. I. Calculation of 0–0 Excitation Energies of Organic Molecules by CIS(D) Quantum Chemical Methods. *Chem. Phys.* **2004**, *305*, 223–230.

(19) Loos, P.-F.; Scemama, A.; Blondel, A.; Garniron, Y.; Caffarel, M.; Jacquemin, D. A Mountaineering Strategy to Excited States: Highly-Accurate Reference Energies and Benchmarks. *J. Chem. Theory Comput.* **2018**, *14*, 4360–4379.

(20) Loos, P. F.; Lipparini, F.; Boggio-Pasqua, M.; Scemama, A.; Jacquemin, D. A Mountaineering Strategy to Excited States: Highly-Accurate Energies and Benchmarks for Medium Size Molecules. *J. Chem. Theory Comput.* **2020**, submitted.

(21) Trofimov, A. B.; Stelter, G.; Schirmer, J. Electron Excitation Energies Using a Consistent Third-Order Propagator Approach: Comparison with Full Configuration Interaction and Coupled Cluster Results. *J. Chem. Phys.* **2002**, *117*, 6402–6410.

(22) Winter, N. O. C.; Graf, N. K.; Leutwyler, S.; Hättig, C. Benchmarks for 0–0 Transitions of Aromatic Or-

ganic Molecules: DFT/B3LYP, ADC(2), CC2, SOS-CC2 and SCS-CC2 Compared to High-resolution Gas-Phase Data. *Phys. Chem. Chem. Phys.* **2013**, *15*, 6623–6630.

(23) Harbach, P. H. P.; Wormit, M.; Dreuw, A. The Third-Order Algebraic Diagrammatic Construction Method (ADC(3)) for the Polarization Propagator for Closed-Shell Molecules: Efficient Implementation and Benchmarking. *J. Chem. Phys.* **2014**, *141*, 064113.

(24) Loos, P. F.; Jacquemin, D. Is ADC(3) as Accurate as CC3 for Valence and Rydberg Transition Energies? *J. Phys. Chem. Lett.* **2020**, *11*, 974–980.

(25) Köhn, A.; Hättig, C. Analytic Gradients for Excited States in the Coupled-Cluster Model CC2 Employing the Resolution-Of-The-Identity Approximation. *J. Chem. Phys.* **2003**, *119*, 5021–5036.

(26) Hellweg, A.; Grün, S. A.; Hättig, C. Benchmarking the Performance of Spin-Component Scaled CC2 in Ground and Electronically Excited States. *Phys. Chem. Chem. Phys.* **2008**, *10*, 4119–4127.

(27) Schreiber, M.; Silva-Junior, M. R.; Sauer, S. P. A.; Thiel, W. Benchmarks for Electronically Excited States: CASPT2, CC2, CCSD and CC3. *J. Chem. Phys.* **2008**, *128*, 134110.

(28) Tajti, A.; Szalay, P. G. Investigation of the Impact of Different Terms in the Second Order Hamiltonian on Excitation Energies of Valence and Rydberg States. *J. Chem. Theory Comput.* **2016**, *12*, 5477–5482.

(29) Loos, P.-F.; Galland, N.; Jacquemin, D. Theoretical 0–0 Energies with Chemical Accuracy. *J. Phys. Chem. Lett.* **2018**, *9*, 4646–4651.

(30) Loos, P.-F.; Jacquemin, D. Chemically Accurate 0-0 Energies with not-so-Accurate Excited State Geometries. *J. Chem. Theory Comput.* **2019**, *15*, 2481–2491.

(31) Schapiro, I.; Sivalingam, K.; Neese, F. Assessment of *n*-Electron Valence State Perturbation Theory for Vertical Excitation Energies. *J. Chem. Theory Comput.* **2013**, *9*, 3567–3580.

(32) Hoyer, C. E.; Ghosh, S.; Truhlar, D. G.; Gagliardi, L. Multiconfiguration Pair-Density Functional Theory Is as Accurate as CASPT2 for Electronic Excitation. *J. Phys. Chem. Lett.* **2016**, *7*, 586–591.

(33) Zobel, J. P.; Nogueira, J. J.; Gonzalez, L. The IPEA Dilemma in CASPT2. *Chem. Sci.* **2017**, *8*, 1482–1499.
